# Supplementary material for: Mobile-URSONet: an Embeddable Neural Network for Onboard Spacecraft Pose Estimation
Source: arXiv:2205.02065 source file (2022-05-04)
Supplement: Supplementary file 1 [file 6-appendix.tex]

\section*{APPENDIX}

%Empty
